# Supplementary material for: PAGED: A Benchmark for Procedural Graphs Extraction from Documents
Source: arXiv:2408.03630 source file (2024-08-08)
Supplement: Supplementary file 1 [file TermDefinition.tex]

\begin{table*}[t]
\caption{Definitions of the terms in the procedural graphs.
}
\label{tab:TermDefinition}
\centering
\scalebox{0.9}{
\begin{tabular}{|c|c|l|}
\hline
\textbf{Term}     & \textbf{Type} & \textbf{Explanation}                                                                                                                                                                \\ \hline
Start             & Node          & the start node indicates the start of the procedure                                                                                                                                 \\ \hline
End               & Node          & the end node indicates the procedure comes to an end                                                                                                                                \\ \hline
Action            & Node          & the action indicates a step to execute in the procedure                                                                                                                             \\ \hline
Exclusive Gateway & Node          & \makecell[l]{designed to represent the branches when the next one action to be executed is \\ determined by specific conditions}                                                                     \\ \hline
Inclusive Gateway & Node          & \makecell[l]{designed to represent the branches when more than one action of the branches \\ can be executed if multiple conditions are satisfied at the same time}                                  \\ \hline
Parallel Gateway  & Node          & designed to represent actions that are executed simultaneously                                                                                                                      \\ \hline
Data Constraint   & Node          & \makecell[l]{explain the constraints for the data requirements of the actions in the procedure \\ which necessitate access to the data objects}                                                      \\ \hline
Action Constraint & Node          & crucial notices need to be considered for the execution of the actions                                                                                                              \\ \hline
Sequence Flow   & Edge          & \makecell[l]{edges used to show the flow of the entire procedure, and can be with specific \\ conditions when representing branches that are executed based on the \\ satisfaction of the conditions} \\ \hline
Constraint Flow   & Edge          & \makecell[l]{edges used to connect action nodes and corresponding Data Constraint or \\ Action Constraint nodes}                                                                                     \\ \hline
Actor             & Attribute     & actor indicates who performs the actions in the procedures if necessary                                                                                                             \\ \hline
\end{tabular}
}
\end{table*}
